# Supplementary material for: Optical conductivity study of screening of many-body effects in graphene interfaces
Source: arXiv:1206.6707 source file (2012-06-29)
Supplement: Supplementary file 1 [file PranjalGogoi_ScreeningInGraphene_SupportingOnlineMaterial.pdf]

**Supporting Online Material**

# Optical conductivity study of screening of many-body effects in graphene interfaces

Pranjal Kumar Gogoi[1,2,3], Iman Santoso[1,3,4], Surajit Saha[1,2], Sihao Wang[2], Antonio H. Castro Neto[2,4], Kian Ping Loh[1,4,5], T. Venkatesan[1,2,6], Andrivo Rusydi[1,2,3,*]

[1]NUSNNI-NanoCore, National University of Singapore, Singapore 117576

[2]Department of Physics, National University of Singapore, Singapore 117542

[3]Singapore Synchrotron Light Source, National University of Singapore, 5 Research Link, Singapore 117603, Singapore

[4]Graphene Research Centre, Faculty of Science, National University of Singapore, Singapore 117546

[5]Department of Chemistry, National University of Singapore, Singapore 117543

[6]Department of Electrical and Computer Engineering, National University of Singapore, Singapore 117576

*phyandri@nus.edu.sg

## A. Sample preparation and Raman measurement

Graphene samples, which were prepared by CVD method on copper foil as reported by Li et al.[1], procured from Graphene Square Inc are used for this study. The thickness of the copper foil is 25 μm. In our laboratory the transfer of the graphene layer to other substrates (amorphous quartz in this work) is performed using a 3-step method[2] –(i) spin coating a PMMA layer on the graphene surface for support and later etching of the back side graphene layer by oxygen-argon plasma; (ii) Etching of the copper layer using 0.1M ammonium persulphate solution $(NH_4)_2S_2O_5$ and (iii) Transfer of graphene layer to substrate (amorphous quartz) and removal of the PMMA layer by acetone treatment.

As shown in Figure S1 below, Raman measurement on the graphene sample on quartz shows very distinct single layer features[3] with minor defect contribution. As shown in Figure S9 and in the Figure 1(a) (main article) the general features and shape of optical conductivity are very similar to exfoliated one with slightly lower value[4].

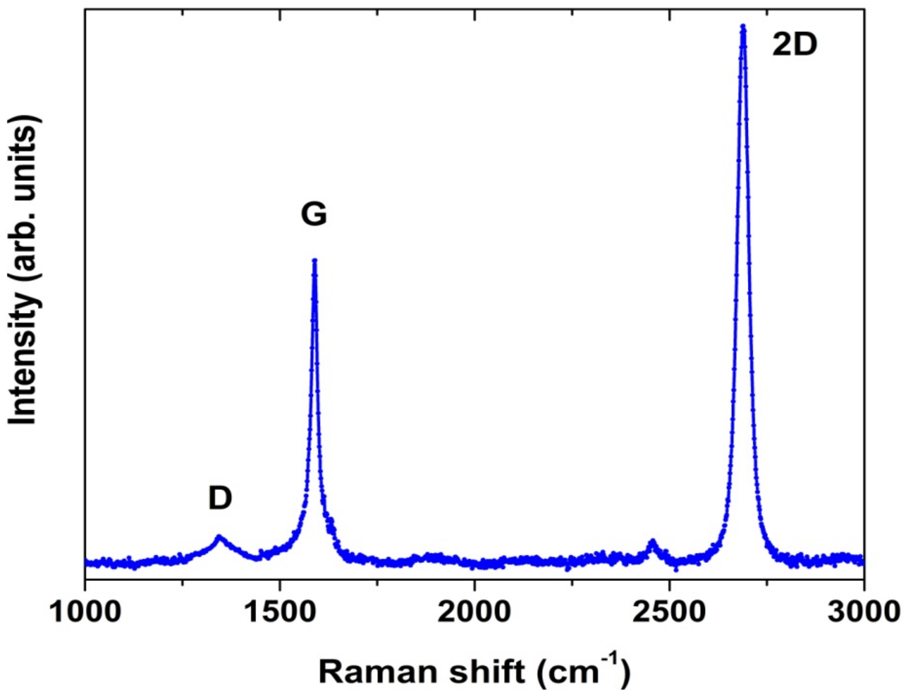


**Figure S1:** Raman Spectra of graphene on quartz 514.5 nm laser

## B. Spectroscopic Ellipsometry Measurement

Spectroscopic ellipsometry[6] measurements are performed on the samples using a SENTECH SE850 ellipsometer. This ellipsometer is equipped with three different light sources—Deep UV( deuterium), UV/VIS source (Xe-lamp) and the NIR source (Halogen lamp of the FT-IR spectrometer) allowing us to measure from 0.5 eV to 6.3 eV. For our measurements we used additional micro-focus probes (~200 micron spot diameter) which work well below 5.3 eV. Therefore this report includes data in the photon energy range from 0.5 – 5.3 eV.

Spectroscopic ellipsometric directly measures the changes of amplitude ratio ($\Psi$) and phase shift ($\Delta$) of *p*- and *s*- component. These parameters, $\Psi$ and $\Delta$, are taken at multiple incident angles and at several spots on the samples. We find that the data at different spots are identical in almost all cases which show sample homogeneity. The multiple incident angle data is used for global fitting of data. A great advantage of spectroscopic ellipsometry measurement is that it directly measures both the real and imaginary parts of the dielectric function together whereas other techniques such as direct reflectivity measurements, required Kramers-Kronig transformation. Furthermore, in a case of very thin films the change in phase of the incident light waves upon reflection is much more pronounced than the change in amplitude of the light of different polarizations. These two facts make ellipsometry an ideal method for analyzing systems like very thin monolayer of graphene on a substrate.

The spectroscopy ellipsometry measurements are done and analyzed as follows. From the same piece of copper foil with graphene (used for transfer to quartz substrate) 5 mm x 5 mm pieces are cut with a sharp blade. Half of those are treated with oxygen argon plasma to remove the graphene layers from their top. Generally in ambient condition copper is always covered with native oxides CuO and $Cu_2O$[5]. In our case treatment in oxygen environment has augmented the process of dominance of CuO with negligible presence of $Cu_2O$. (Also later, fitting procedure shows that the measured spectral spectroscopic ellipsometry data requires only CuO contribution to fit with no contribution from $Cu_2O$ to further confirm this.). The plasma-treated Cu foils are kept in ultrasonic bath for 30 minutes submerged in ethanol to remove the unwanted oxide layer of CuO from its surface[5]. We observe some systematic increase in the pseudo-dieletric functions upon spectroscopic ellipsometry measurement in between of the copper foil with the increase in ultra-sonification time reaching saturation values for 30 minutes and beyond. Spectroscopic

ellipsometry data of Ψ and Δ are taken on these copper foils as well as on those with graphene on copper. Graphene was grown on pure and clean copper. The dielectric function of pure copper is extracted by fitting the Ψ and Δ simultaneously with a multilayer model of a thin layer CuO (which remains even after ultrasonication in ethanol) on top of pure copper. This is later used for fitting of the psi delta data measured on graphene on top of copper.

In Figure S2 we show the measured Ψ and Δ values of samples with graphene and without graphene on substrate (quartz and copper, respectively) at 70 degree incident angle. The spectra show the pronounced contrast due to the presence of graphene which is only ~3 angstrom thick.

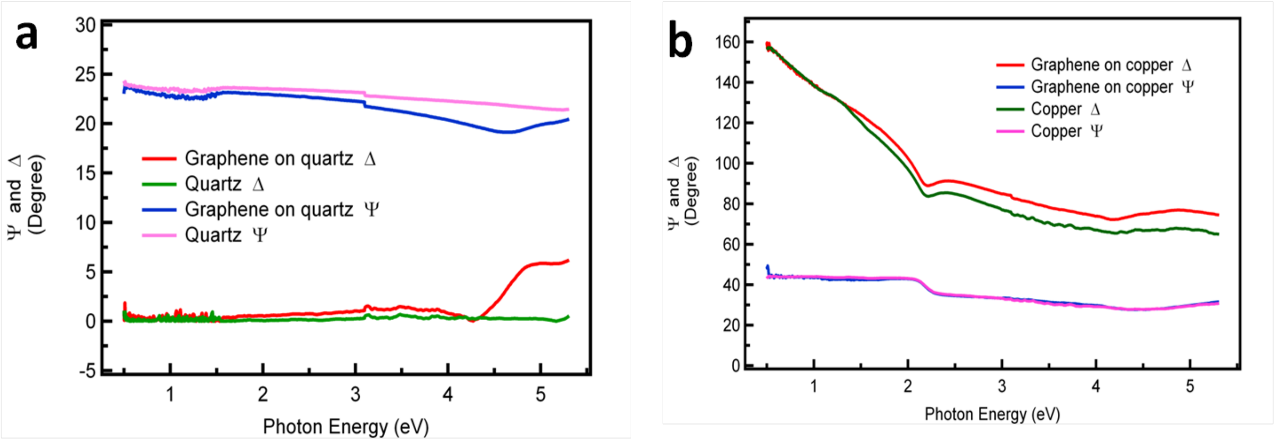


**Figure S2:** (a) Δ and ψ plots of graphene on quartz (GOQ) and pure quartz taken using spectroscopic ellipsometer at 70 degree incident angle. (b) Δ and ψ plots of graphene on copper (GOC) and copper foil taken using spectroscopic ellipsometer at 70 degree incident angle.

## C. <u>Data Analysis:</u>

To extract the dielectric function of the graphene layer, multilayer modeling is performed which takes into account reflections at each interface through Fresnel coefficients. The graphene layer has been assumed to be flat and isotropic[7, 8]. We have used global fitting with simultaneous fitting of data for two incident angles (60 and 70 degrees) both for graphene on quartz and for graphene on copper to get the unique dielectric functions. The fitting is performed using Drude-Lorentz oscillator models in all cases.

Figure S3 shows the plots of fitting for the $\varepsilon_1$ and $\varepsilon_2$ values found from the direct conversion of the $\Psi$ and $\Delta$ values measured on the bulk quartz substrate. This conversion is direct as the substrate (quartz) is bulk. In all subsequent fittings multilayer models have to be used due to the presence of thin layers on top of the substrate- in which case the direct numerical inversion is not straightforward. The multilayer model and fitting result of graphene of quartz (GOQ) are shown in shown in Figure S4. Finally the optical conductivity, $\sigma_1(\omega)$, for only the graphene layer (separated from quartz) is plotted in Figure S5.

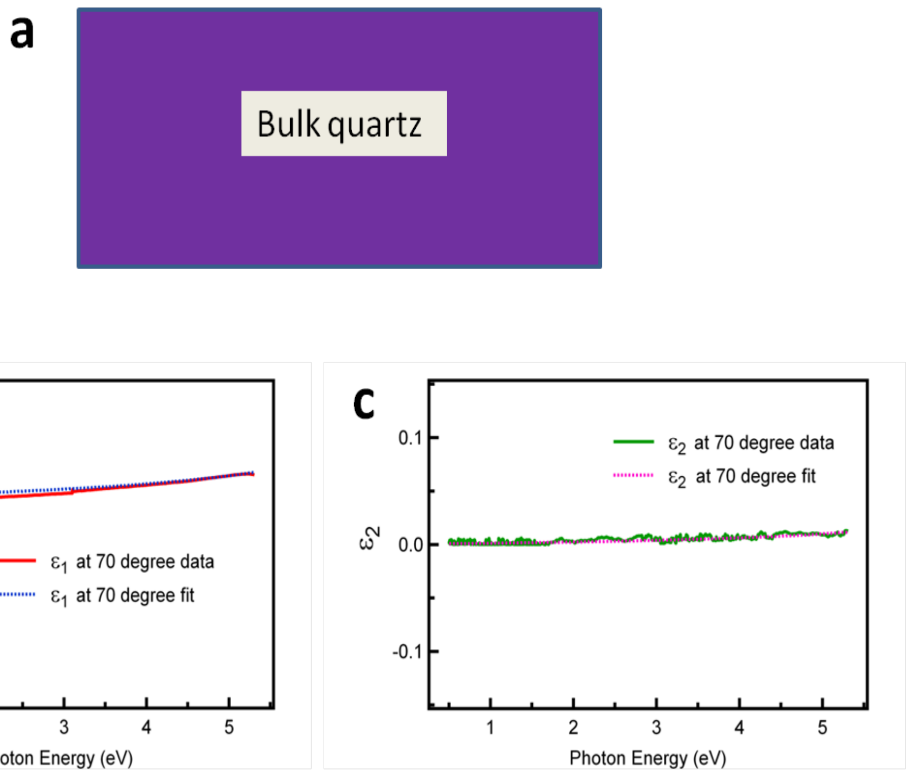


**Figure S3:** (a) Bulk substrate model for quartz. (b) Fitting of $\varepsilon_1$ at 70 degree incident angle for quartz. (c) Fitting of $\varepsilon_2$ at 70 degree incident angle for quartz.

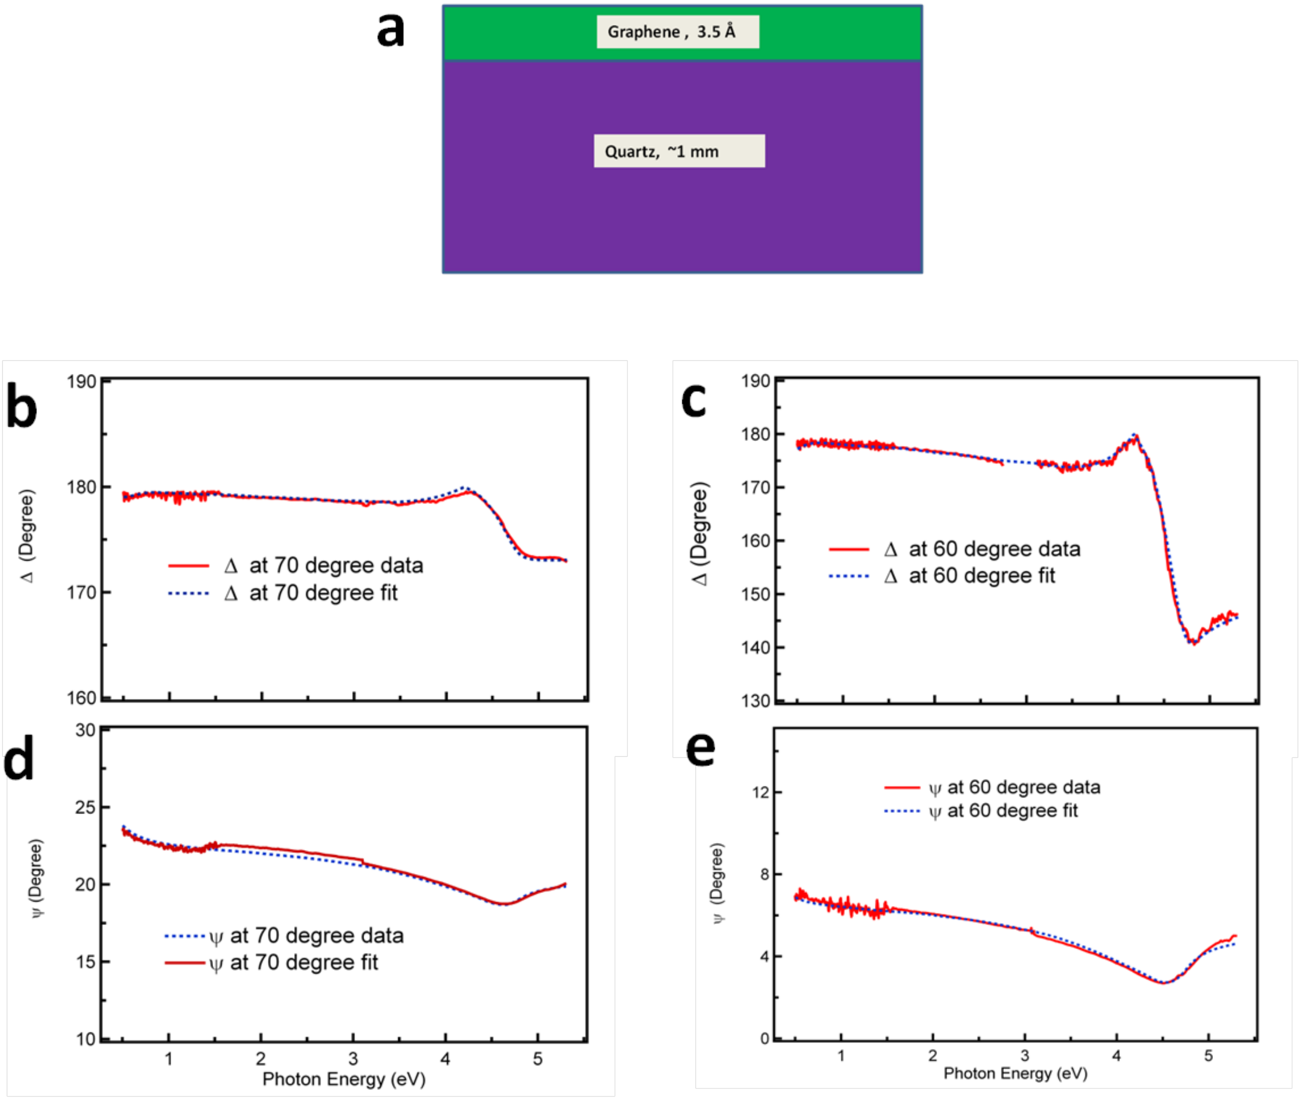


**Figure S4:** (a) Multilayer model for graphene on quartz (GOQ). (b) Fitting of Δ at 70 degree incident angle for graphene on quartz (GOQ). (c) Fitting of Δ at 60 degree for graphene on quartz (GOQ). The data around 3.2 eV are not reliable here due to the detector sensitivity issues. Therefore not shown from ~2.6 to 3.3 eV. (d) Fitting of ψ at 70 degree for graphene on quartz (GOQ). (e) Fitting of ψ at 60 degree for graphene on quartz (GOQ).

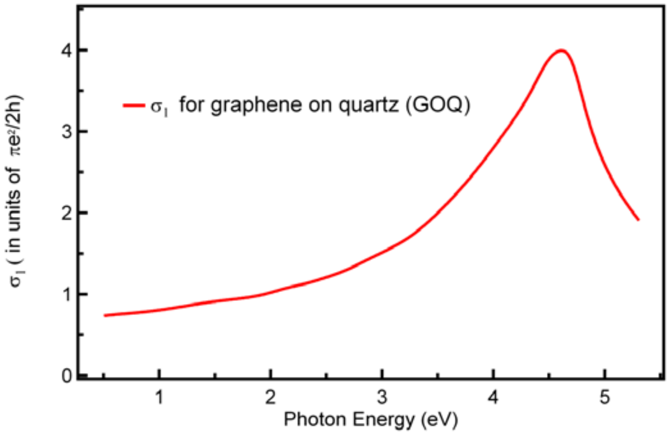


**Figure S5:** Extracted optical conductivity ($\sigma_1$) of graphene on quartz (GOQ)

To extract the optical conductivity, $\sigma_1(\omega)$ of graphene layer on copper (GOC) we proceed similarly as in case of GOQ above. But here we have to extract the pure copper dielectric function first using the multilayer model for the copper substrate itself due to the presence of CuO layer. For the dielectric function used for CuO we find that we can use the same oscillator positions as used by Ito et al. (1-5 eV)[9] with slightly different strengths but with similar overall final structure. The oscillators parameters are listed in Table S1. Differences in crystal structure, growth conditions and surface coverage may be the reasons of these variations. We get the best fit for our data using the results shown in Figures S6(f) and S6(g). Similarly our copper result shown in Figures 6(e) and 6(f) is similar in structure to reported values[10, 11].

| Serial number | $W_0$ (in $cm^{-1}$) | $W_p$ (in $cm^{-1}$) | Width (in $cm^{-1}$) |
|---|---|---|---|
| 1 | 12900 | 907.22 | 1231.2 |
| 2 | 16120 | 11490 | 5572.3 |
| 3 | 20900 | 16783 | 6770.9 |
| 4 | 27000 | 21737 | 9214.5 |
| 5 | 64922 | 141240 | 61406 |

**Table S1**: Drude-Lorentz parameters for dielectric function

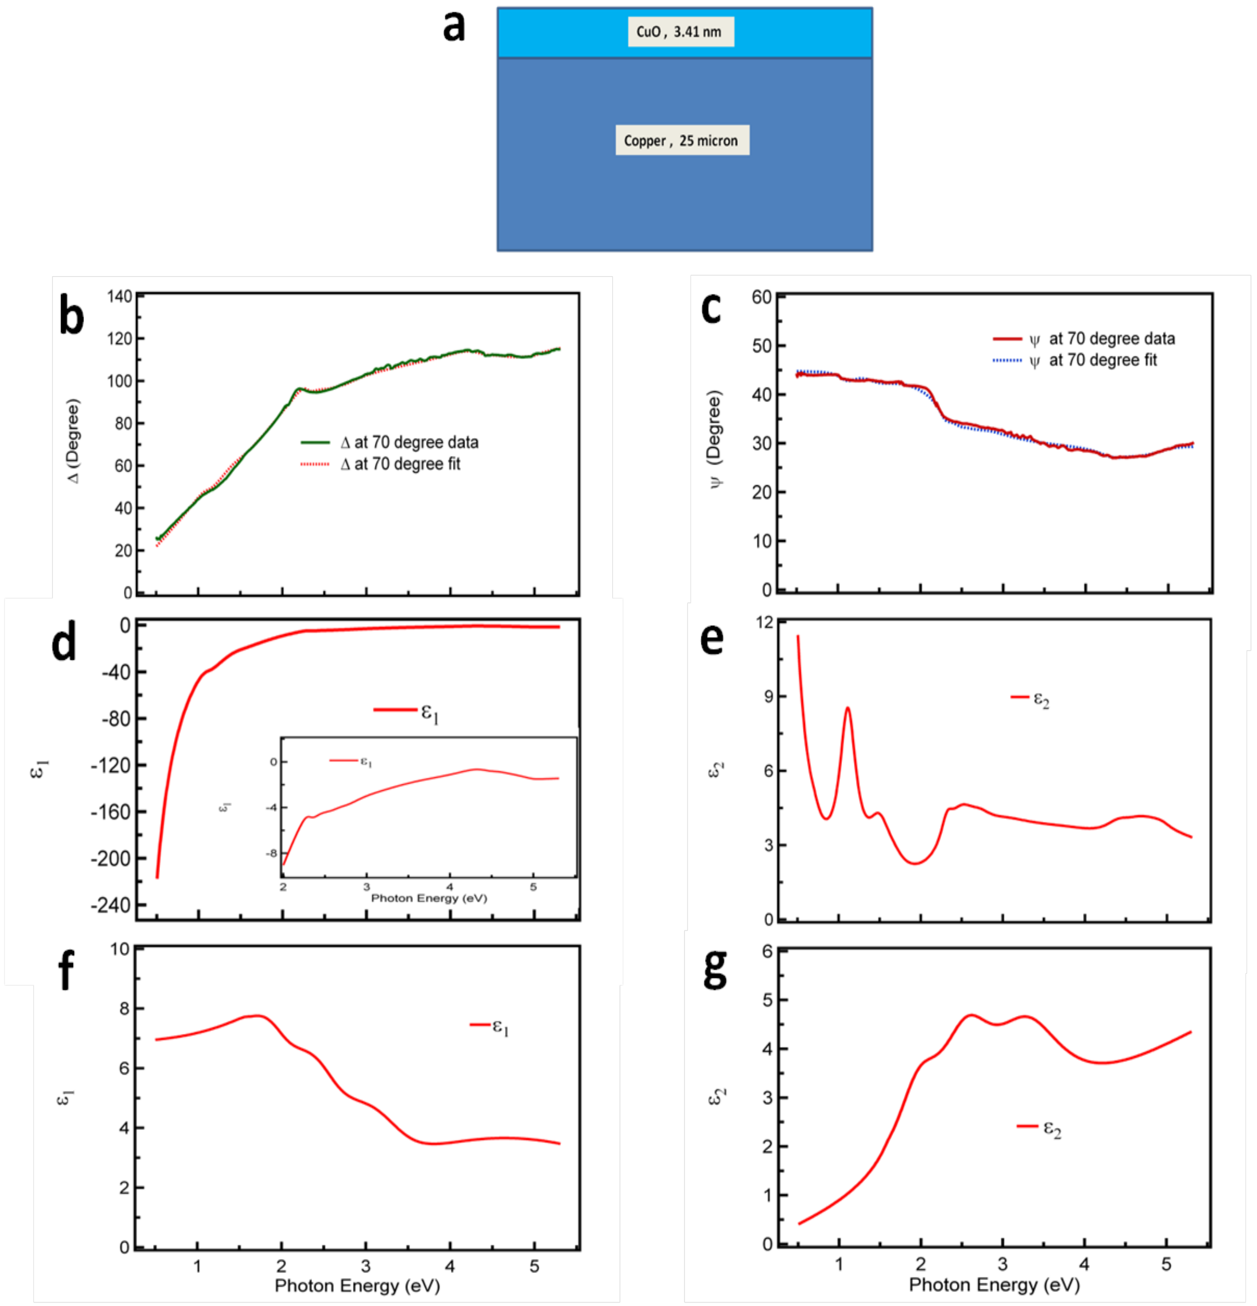


**Figure S6:** (a) Multilayer model of CuO on copper. (b) Fitting of Δ ψ at 70 degree for copper. (c) Fitting of ψ at 70 degree for copper . (d) Extracted $\varepsilon_1$ for copper. (e) Extracted $\varepsilon_2$ for copper. (f) Extracted $\varepsilon_1$ for CuO. (g) Extracted $\varepsilon_2$ for CuO.

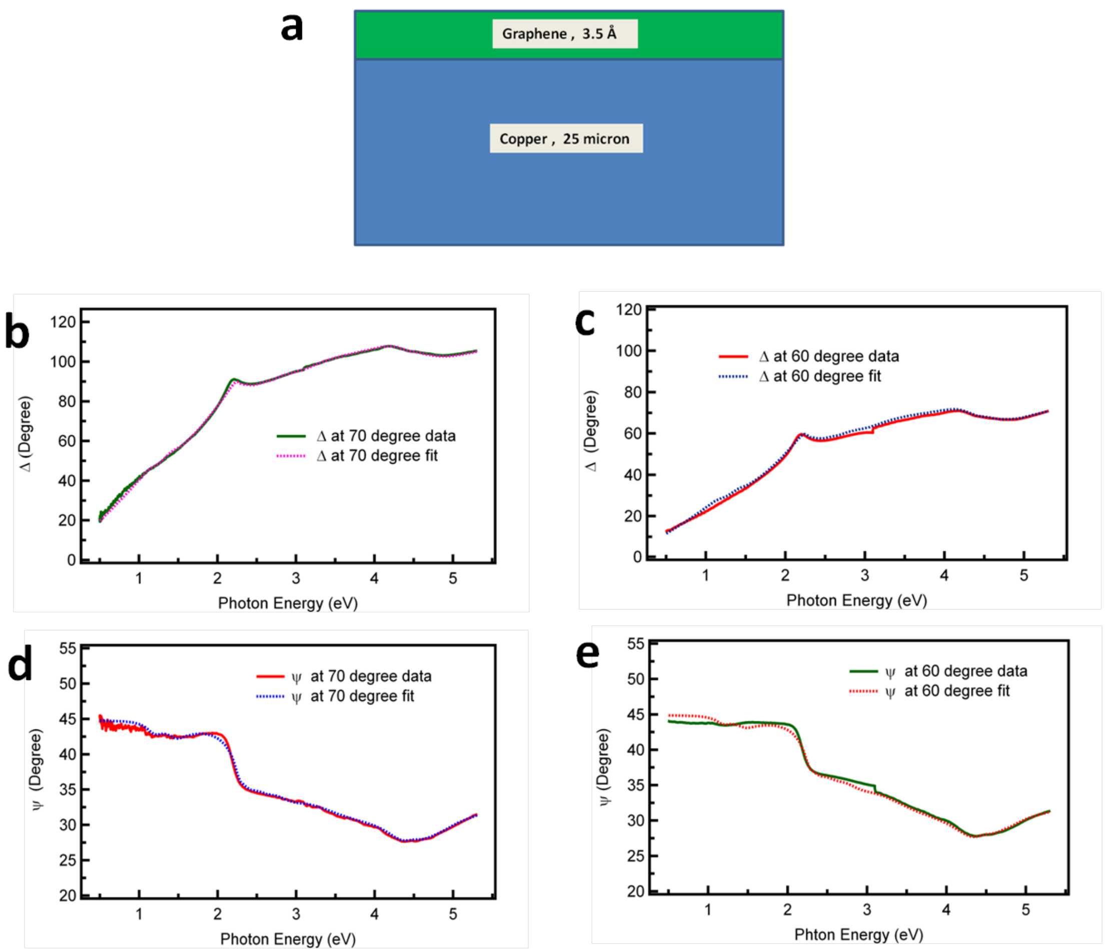


**Figure S7:** (a) Multilayer model of graphene on copper (GOC) (b) Fitting of $\Delta$ at 70 degree incident angle for graphene on copper (GOC). (c) Fitting of $\Delta$ at 60 degree for graphene on copper (GOC). (d) Fitting of $\psi$ at 70 degree for graphene on copper (GOC). (e) Fitting of $\psi$ at 60 degree for graphene on copper (GOC).

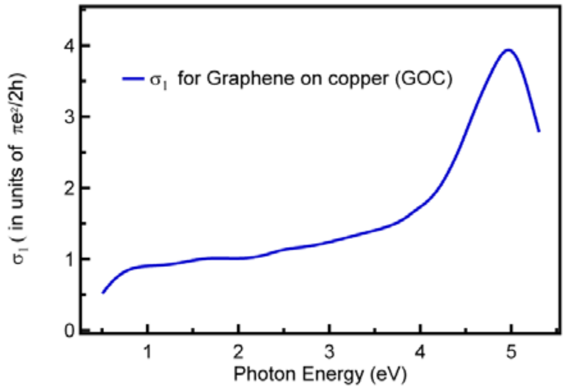


**Figure S8:** Extracted optical conductivity ($\sigma_1$) of graphene on copper (GOC).

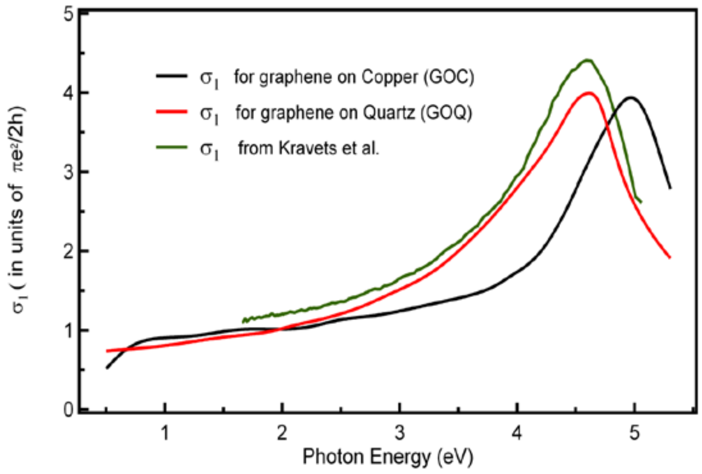


**Figure S9:** Comparison of optical conductivity ($\sigma_1$) for graphene on copper (GOC) and graphene on quartz (GOQ) with comparison with Ref. [4].

## D. Fano line-shape analysis

In Fano analysis[12], the relationship between the final optical conductivity $\sigma_1(\omega)$ and the unperturbed $\sigma_{cont}(\omega)$ can be expressed as

$$\frac{\sigma(\omega)}{\sigma_{cont}(\omega)} = C\frac{(q+\varepsilon)^2}{1+\varepsilon^2} \qquad (1)$$

Here $\varepsilon = (\omega - \omega_{res})/(\Gamma/2)$ is the normalized energy by width $\Gamma$ relative to the excitonic resonance energy $\omega_{res}$. The magnitude of $q^2$ quantifies the ratio of the strength of the e-h coupling to the band to band transition, whereas the asymmetry of the line-shape is determined by the sign of q.

For the band to band transitions of a single particle we use an approach similar to Phillips [13, 14] and also used recently by Chae et al.[15]. Here we take the joint density of states (JDOS) near the saddle point singularity

$$\sigma_{cont}(\omega) \sim -\log|1-\omega/\omega_0|$$

For our data for GOQ we have used

$$\sigma_{cont,GOQ}(\omega) = (-1.7)\log|1-\omega/\omega_0| + C_{GOQ} \qquad (2)$$

which gives the best fit for our data. Similarly for our data for GOC we have used

$$\sigma_{cont,GOC}(\omega) = (-1.7)\log|1-\omega/\omega_0| + C_{GOC} \qquad (3)$$

which gives the best fit for our data. This unperturbed $\boldsymbol{\sigma_{cont}}(\omega)$ is convoluted with a Gaussian of width 380 meV to account for the experimental broadening. The background constant values of 0.68 for $\boldsymbol{C_{GOQ}}$ and 0.76 for $\boldsymbol{C_{GOC}}$ are added to account for the constant σ($\omega$) in the infrared and visible energy range (universal constant σ($\omega$) for the ideal graphene).

The results of the Fano fitting of σ($\omega$) for GOQ are plotted in Fig 2(a) of the main article. The Fano parameters for GOQ are q = -1.16, Γ = 0.99 eV and $E_{res} = 4.90$ eV. These numbers are comparable to the reported values for exfoliated graphene. Particularly the large value Γ signifies a short life-time (~0.34 fs). The reasonable fitting to Fano model signifies the presence of prominent excitonic effects in our graphene sample, GOQ. For GOC, the Fano parameters are q = -0.96, Γ = 0.98 eV and $E_{res} = 5.19$ eV. These parameters can only account for the redshift from the unperturbed peak at 5.2 eV but not the symmetric shape of our result of GOC.

**References:**


1. Li, X., Cai, W., An, J., Kim, S., Nah, J., Yang, D., Piner, R., Velamakanni, A., Jung, I., Tutuc, E., Banerjee, S. K., Colombo, L., Ruoff, R. S. Large-Area Synthesis of High-Quality and Uniform Graphene Films on Copper Foils. *Science* 324, 1312 (2009).

2. Bae, S., Hyeongkeun, K., Lee, Y., Xiangfan, X., Park, J. S., Yi, Z., Balakrishnan, J., Lei, T., Kim, H. R., Song, Y., Kim, Y. J., Kim, K. S., Oezyilmaz, B., Ahn, J. H., Hong B. H., Iijima, S. Roll-to-roll production of 30-inch graphene films for transparent electrodes. *Nature Nanotech*. 5, 574 (2010).

3. Ferrari, A. C., Meyer, J. C., Scardaci, V. , Casiraghi, C. , Lazzeri, M., Mauri, F., Piscanec, S., Jiang, D., Novoselov, K. S., Roth, S. Geim, A. K. Raman Spectrum of Graphene and Graphene Layers. *Phys. Rev. Lett*. 97, 187401 (2006).

4. Kravets, V. G., Grigorenko, A. N., Nair, R. R., Blake, P., Anissimova, S., Novoselov K.S., Geim, A. K. Spectroscopic ellipsometry of graphene and an exciton-shifted van Hove peak in absorption. *Phys. Rev.* B 81, 155413 (2010).

5. Satta, A., Shamiryan, D., Baklanov, M. R. , Whelan, C. M., Le, Q. T., Beyer, G. P., Vantomme, A., Maex, K. The Removal of Copper Oxides by Ethyl Alcohol Monitored *In Situ* by Spectroscopic Ellipsometry. *J. Electrochem. Soc.* 150, 5, G300-G306 (2003)

6. Azzam R. M. A., Bashara, N. M. *Ellipsometry and Polarized Light,* North-Holland, Amsterdam (1977).

7. Nelson, F. J., Kamineni, V. K., Zhang, T., Comfort, E. S., Lee, J. U., Diebold, A. C. Optical properties of large-area polycrystalline chemical vapor deposited graphene by spectroscopic ellipsometry. *Appl. Phys. Lett*., 97, 253110 (2010).

8. Weber, J. W., Calado, V. E., van de Sanden, M. C. M. Optical constants of graphene measured by spectroscopic ellipsometry. *Appl. Phys. Lett.*, 97, 091904 (2010).

9. Ito, T., Yamguchi, H., Masumi, T., Adachi, S. Optical Properties of CuO Studied by Spectroscopic Ellipsometry. *J. Phys. Soc. of Japan*, 67, 9, 3304-3309 (1998).

10. E. D. Palik, Editor, *Handbook of Optical Constants of Solids II*, Academic Press, New York (1991).

11. Ehrenreich, H., Philipp H. R. Optical properties of Ag and Cu. *Phys. Rev*. 128, 4, 1622 (1962).

12. Fano, U. Effects of Configuration Interaction on Intensities and Phase Shifts. *Phys. Rev*. 124, 6, 1866 (1961).

13. Philiips, J. C. Ultraviolet Absorption of Insulators. III. fcc Alkali Halides. *Phys. Rev*. 136, 6A, A1705 (1964).

14. Phillips, J. C. *Excitons. In The Optical Properties of Solids*; Tauc, J., Ed.; Academic Press, New York, (1966).

15. Chae, D. H., Utikal, T., Weisenburger, S., Giessen, H., Klitzing, K. v., Lippitz, M., Smet, J. Excitonic Fano Resonance in Free-Standing Graphene. *Nano. Lett.* 11, 1379–1382 (2011).
